# Supplementary material for: A Continual Learning-driven Model for Accurate and Generalizable Segmentation of Clinically Comprehensive and Fine-grained Whole-body Anatomies in CT
Source: arXiv:2503.12698 source file (2025-03-16)
Supplement: Supplementary file 4 [file tab_supp_tab_dataset-wise_u5_mt.tex]

\begin{table}[htp]
\centering
\fontsize{10pt}{12pt}\selectfont
% \resizebox{\textwidth}{!}{
\begin{tabular}{|l|ll|ll|ll|r|}
\hline
 & \multicolumn{2}{c|}{\ac{nnu_e5}} & \multicolumn{2}{c|}{MultiTalent} & \multicolumn{3}{c|}{\ac{cln_u5}} \\ \cline{2-8} 
\multirow{-2}{*}{} & DSC$\uparrow$ & ASD$\downarrow$ & DSC$\uparrow$ & ASD$\downarrow$ & DSC$\uparrow$ & ASD$\downarrow$ & $\mathcal{T}\uparrow$ \\ \hline
\rowcolor[HTML]{F3F3F3} 
Spleen & 97.6$\pm$15.6 & 1.95$\pm$0.40 & 96.6$\pm$3.2 & 0.36$\pm$0.44 & 97.1$\pm$6.8 & 1.65$\pm$0.39 & 99.7 \\
Kidney\_R & 95.9$\pm$16.9 & 0.19$\pm$0.73 & 95.7$\pm$4.7 & 0.29$\pm$0.30 & 96.1$\pm$7.1 & 0.21$\pm$0.76 & 99.7 \\
Kidney\_L & 96.1$\pm$26.7 & 1.15$\pm$6.45 & 91.9$\pm$17.5 & 1.72$\pm$8.64 & 97.2$\pm$6.9 & 1.00$\pm$0.72 & {} \\
\rowcolor[HTML]{F3F3F3} 
GallBladder & 92.2$\pm$24.4 & 1.14$\pm$0.82 & 86.0$\pm$19.3 & 1.42$\pm$2.67 & 93.2$\pm$8.7 & 0.95$\pm$0.83 & 99.7 \\
Liver & 97.3$\pm$14.9 & 0.57$\pm$0.93 & 97.8$\pm$1.5 & 0.52$\pm$0.65 & 97.5$\pm$5.8 & 0.54$\pm$0.93 & 99.5 \\
\rowcolor[HTML]{F3F3F3} 
Stomach & 95.9$\pm$16.2 & 1.18$\pm$0.66 & 94.2$\pm$8.2 & 0.66$\pm$0.68 & 96.5$\pm$6.2 & 1.11$\pm$0.66 & 99.5 \\
Pancreas & 91.8$\pm$17.0 & 1.06$\pm$0.67 & 90.3$\pm$6.8 & 0.79$\pm$1.53 & 92.0$\pm$6.9 & 0.84$\pm$0.37 & 99.5 \\
\rowcolor[HTML]{F3F3F3} 
Glnd\_Adrenal\_R & 83.0$\pm$13.5 & 0.55$\pm$1.17 & 87.8$\pm$11.2 & 0.50$\pm$1.60 & 84.2$\pm$13.3 & 0.43$\pm$0.39 & 94.0 \\
\rowcolor[HTML]{F3F3F3} 
Glnd\_Adrenal\_L & 84.2$\pm$12.2 & 1.03$\pm$0.36 & 85.4$\pm$13.5 & 0.31$\pm$0.26 & 84.8$\pm$12.5 & 0.87$\pm$0.39 & {\cellcolor[HTML]{F3F3F3}} \\
Lung\_LUL & 97.8$\pm$3.6 & 0.31$\pm$0.93 & 97.3$\pm$4.5 & 1.15$\pm$4.41 & 97.9$\pm$3.7 & 0.17$\pm$0.62 & 99.7 \\
Lung\_LLL & 96.5$\pm$24.0 & 0.21$\pm$0.98 & 95.7$\pm$8.5 & 0.72$\pm$1.68 & 96.5$\pm$2.1 & 0.21$\pm$0.47 & {} \\
\rowcolor[HTML]{F3F3F3} 
Lung\_RUL & 97.5$\pm$20.5 & 0.30$\pm$1.48 & 92.0$\pm$19.5 & 0.77$\pm$1.37 & 97.7$\pm$2.5 & 0.20$\pm$0.98 & 99.5 \\
\rowcolor[HTML]{F3F3F3} 
Lung\_RML & 92.0$\pm$6.2 & 0.47$\pm$1.41 & 94.8$\pm$6.5 & 0.83$\pm$1.31 & 92.3$\pm$3.3 & 0.22$\pm$1.50 & {\cellcolor[HTML]{F3F3F3}} \\
\rowcolor[HTML]{F3F3F3} 
Lung\_RLL & 97.4$\pm$26.8 & 0.16$\pm$2.45 & 97.2$\pm$5.9 & 0.43$\pm$0.83 & 97.2$\pm$3.6 & 0.21$\pm$1.19 & {\cellcolor[HTML]{F3F3F3}} \\
Eso & 94.8$\pm$2.9 & 0.61$\pm$0.15 & 94.1$\pm$2.1 & 0.24$\pm$0.24 & 94.4$\pm$3.1 & 0.45$\pm$0.16 & 99.7 \\
\rowcolor[HTML]{F3F3F3} 
Trachea & 96.7$\pm$5.8 & 0.36$\pm$0.12 & 96.0$\pm$5.0 & 0.27$\pm$0.47 & 97.1$\pm$6.1 & 0.27$\pm$0.12 & 99.5 \\
Glnd\_Thyroid & 91.7$\pm$14.7 & 0.41$\pm$0.96 & 90.2$\pm$9.2 & 0.37$\pm$0.45 & 92.6$\pm$14.5 & 0.28$\pm$0.96 & 99.7 \\
\rowcolor[HTML]{F3F3F3} 
SmallBowel & 91.2$\pm$26.4 & 1.63$\pm$2.53 & 87.4$\pm$14.0 & 1.56$\pm$1.77 & 91.2$\pm$16.6 & 1.55$\pm$2.62 & 99.7 \\
Duodenum & 87.3$\pm$26.0 & 1.87$\pm$1.26 & 82.9$\pm$18.3 & 1.02$\pm$1.08 & 88.8$\pm$16.1 & 1.81$\pm$1.26 & 99.5 \\
\rowcolor[HTML]{F3F3F3} 
Colon & 90.2$\pm$16.0 & 2.54$\pm$1.21 & 89.9$\pm$7.9 & 1.55$\pm$1.90 & 90.4$\pm$15.8 & 2.36$\pm$1.23 & 99.5 \\
UrinaryBladder & 89.1$\pm$9.5 & 2.98$\pm$1.08 & 92.5$\pm$7.6 & 1.27$\pm$1.97 & 89.2$\pm$9.6 & 2.85$\pm$1.03 & 99.5 \\
\rowcolor[HTML]{F3F3F3} 
Prostate & 81.7$\pm$38.0 & 0.52$\pm$2.06 & 72.8$\pm$33.5 & 1.45$\pm$1.72 & 83.3$\pm$17.9 & 0.35$\pm$1.47 & 99.5 \\ \hline

Mean & \multicolumn{1}{c}{ 92.6 } & \multicolumn{1}{c|}{ 0.96 } & \multicolumn{1}{c}{ 91.3 } & \multicolumn{1}{c|}{ 0.83 } & \multicolumn{1}{c}{ 93.1 } & \multicolumn{1}{c|}{ 0.84 } & \multicolumn{1}{c|}{ 99.3 } \\ \hline
\end{tabular}
% }
\caption{\textbar~\textbf{Organ-wise performance comparison of \ac{nnu_e5}, MultiTalent, and \ac{cln_u5} on \ac{totalseg} `Organ' subgroup.} Organ-wise DSC (\%) and ASD (mm) of \ac{nnu_e5}, MultiTalent and \ac{cln_u5} are evaluated on \ac{totalseg} `Organ' subgroup. \ac{cln_u5} achieves the best mean DSC.}
\label{tab:pl_totalseg_organ_ds5}
\end{table}
\clearpage

\begin{table}[htp]
\centering
\fontsize{10pt}{12pt}\selectfont
% \resizebox{\textwidth}{!}{
\begin{tabular}{|l|ll|ll|ll|r|}
\hline
 & \multicolumn{2}{c|}{\ac{nnu_e5}} & \multicolumn{2}{c|}{MultiTalent} & \multicolumn{3}{c|}{\ac{cln_u5}} \\ \cline{2-8} 
\multirow{-2}{*}{} & DSC$\uparrow$ & ASD$\downarrow$ & DSC$\uparrow$ & ASD$\downarrow$ & DSC$\uparrow$ & ASD$\downarrow$ & $\mathcal{T}\uparrow$ \\ \hline
\rowcolor[HTML]{F3F3F3} 
Heart & 95.2$\pm$14.7 & 0.42$\pm$0.20 & 95.9$\pm$1.4 & 1.10$\pm$3.24 & 94.9$\pm$14.7 & 0.43$\pm$0.18 & \multicolumn{1}{r|}{\cellcolor[HTML]{F3F3F3}99.7} \\
A\_Aorta & 96.0$\pm$16.7 & 0.44$\pm$0.95 & 96.7$\pm$4.7 & 0.30$\pm$0.57 & 96.5$\pm$16.7 & 0.41$\pm$0.85 & \multicolumn{1}{r|}{99.7} \\
\rowcolor[HTML]{F3F3F3} 
V\_Pulmonary & 89.8$\pm$15.5 & 0.47$\pm$0.14 & 93.1$\pm$3.1 & 0.23$\pm$0.13 & 91.3$\pm$15.5 & 0.31$\pm$0.16 & \multicolumn{1}{r|}{\cellcolor[HTML]{F3F3F3}99.0} \\
A\_BrachiocephalicTrunk & 89.8$\pm$16.2 & 0.32$\pm$0.43 & 93.8$\pm$3.0 & 0.22$\pm$0.18 & 90.8$\pm$16.3 & 0.22$\pm$0.44 & \multicolumn{1}{r|}{99.0} \\
\rowcolor[HTML]{F3F3F3} 
A\_Subclavian\_L & 94.6$\pm$3.5 & 0.44$\pm$0.28 & 91.6$\pm$3.5 & 0.33$\pm$0.47 & 94.9$\pm$3.6 & 0.27$\pm$0.29 & 99.7 \\
\rowcolor[HTML]{F3F3F3} 
A\_Subclavian\_R & 94.1$\pm$3.3 & 0.23$\pm$0.17 & 91.5$\pm$3.4 & 0.22$\pm$0.15 & 93.3$\pm$3.4 & 0.17$\pm$0.18 & {\cellcolor[HTML]{F3F3F3}} \\
A\_CommonCarotid\_L & 91.2$\pm$5.4 & 0.35$\pm$0.28 & 90.3$\pm$4.8 & 0.23$\pm$0.22 & 91.1$\pm$5.4 & 0.24$\pm$0.28 & 99.5 \\
A\_CommonCarotid\_R & 96.6$\pm$3.3 & 0.28$\pm$0.99 & 93.2$\pm$2.4 & 0.15$\pm$0.13 & 97.4$\pm$3.3 & 0.26$\pm$1.02 & {} \\
\rowcolor[HTML]{F3F3F3} 
V\_Brachiocephalic\_L & 90.4$\pm$26.2 & 0.37$\pm$1.97 & 91.5$\pm$15.7 & 0.44$\pm$1.59 & 91.2$\pm$16.1 & 0.31$\pm$2.11 & 99.5 \\
\rowcolor[HTML]{F3F3F3} 
V\_Brachiocephalic\_R & 88.7$\pm$15.0 & 0.32$\pm$0.81 & 89.8$\pm$11.4 & 0.37$\pm$0.57 & 89.1$\pm$15.3 & 0.24$\pm$0.84 & {\cellcolor[HTML]{F3F3F3}} \\
LAA & 92.6$\pm$3.4 & 0.46$\pm$0.15 & 93.2$\pm$2.7 & 0.20$\pm$0.11 & 91.7$\pm$3.3 & 0.16$\pm$0.15 & 99.5 \\
\rowcolor[HTML]{F3F3F3} 
V\_VenaCava\_S & 93.8$\pm$21.4 & 0.23$\pm$2.35 & 88.4$\pm$24.2 & 0.42$\pm$0.83 & 93.7$\pm$21.4 & 0.18$\pm$2.44 & 99.5 \\
V\_VenaCava\_I & 93.9$\pm$9.8 & 1.03$\pm$1.05 & 92.3$\pm$6.3 & 0.47$\pm$0.38 & 95.2$\pm$9.8 & 0.77$\pm$1.00 & 99.5 \\
\rowcolor[HTML]{F3F3F3} 
V\_Portal\_Splenic & 85.5$\pm$29.3 & 1.29$\pm$0.62 & 85.1$\pm$12.1 & 0.67$\pm$0.72 & 86.7$\pm$29.1 & 1.12$\pm$0.63 & 99.0 \\
A\_Iliac\_L & 94.4$\pm$3.1 & 0.61$\pm$0.19 & 93.2$\pm$3.0 & 0.25$\pm$0.38 & 95.1$\pm$3.3 & 0.50$\pm$0.20 & 99.5 \\
A\_Iliac\_R & 91.9$\pm$19.5 & 0.45$\pm$0.15 & 93.5$\pm$3.8 & 0.19$\pm$0.26 & 91.9$\pm$19.6 & 0.39$\pm$0.18 & {} \\
\rowcolor[HTML]{F3F3F3} 
V\_Iliac\_L & 92.2$\pm$3.0 & 0.48$\pm$0.13 & 94.1$\pm$2.8 & 0.18$\pm$0.10 & 92.9$\pm$3.3 & 0.43$\pm$0.15 & 99.0 \\
\rowcolor[HTML]{F3F3F3} 
V\_Iliac\_R & 94.2$\pm$4.9 & 0.44$\pm$0.31 & 92.9$\pm$5.6 & 0.22$\pm$0.20 & 93.6$\pm$4.8 & 0.45$\pm$0.27 & {\cellcolor[HTML]{F3F3F3}}
\\ \hline

Mean & \multicolumn{1}{c}{ 92.5 } & \multicolumn{1}{c|}{ 0.48 } & \multicolumn{1}{c}{ 92.2 } & \multicolumn{1}{c|}{ 0.34 } & \multicolumn{1}{c}{ 92.9 } & \multicolumn{1}{c|}{ 0.38 } & \multicolumn{1}{c|}{ 99.4 } \\ \hline

\end{tabular}
% }
\caption{\textbar~\textbf{Organ-wise performance comparison of \ac{nnu_e5}, MultiTalent, and \ac{cln_u5} on \ac{totalseg} `Cardiac' subgroup.} Organ-wise DSC (\%) and ASD (mm) of \ac{nnu_e5}, MultiTalent and \ac{cln_u5} are evaluated on \ac{totalseg} `Cardiac' subgroup. \ac{cln_u5} achieves the best mean DSC.}
\label{tab:pl_totalseg_cardi_ds5}
\end{table}
\clearpage

\begin{table}[htp]
\centering
\fontsize{10pt}{12pt}\selectfont
% \resizebox{\textwidth}{!}{
\begin{tabular}{|l|ll|ll|ll|r|}
\hline
 & \multicolumn{2}{c|}{\ac{nnu_e5}} & \multicolumn{2}{c|}{MultiTalent} & \multicolumn{3}{c|}{\ac{cln_u5}} \\ \cline{2-8} 
\multirow{-2}{*}{} & DSC$\uparrow$ & ASD$\downarrow$ & DSC$\uparrow$ & ASD$\downarrow$ & DSC$\uparrow$ & ASD$\downarrow$ & $\mathcal{T}\uparrow$ \\ \hline
\rowcolor[HTML]{F3F3F3} 
Bone\_Humerus\_L & 96.9$\pm$17.5 & 2.84$\pm$0.20 & 93.5$\pm$7.1 & 0.57$\pm$0.97 & 97.1$\pm$17.6 & 2.77$\pm$0.21 & \multicolumn{1}{r|}{\cellcolor[HTML]{F3F3F3}99.5} \\
\rowcolor[HTML]{F3F3F3} 
Bone\_Humerus\_R & 96.6$\pm$17.3 & 4.31$\pm$0.17 & 96.5$\pm$2.0 & 5.20$\pm$12.27 & 97.1$\pm$17.0 & 3.88$\pm$0.17 & \multicolumn{1}{l|}{\cellcolor[HTML]{F3F3F3}} \\
Bone\_Scapula\_L & 94.1$\pm$21.1 & 1.16$\pm$0.18 & 94.8$\pm$1.9 & 0.49$\pm$1.16 & 93.8$\pm$21.4 & 0.97$\pm$0.17 & 99.5 \\
Bone\_Scapula\_R & 95.1$\pm$1.7 & 1.95$\pm$0.07 & 95.2$\pm$2.1 & 0.35$\pm$0.59 & 94.4$\pm$1.9 & 1.63$\pm$0.08 & {} \\
\rowcolor[HTML]{F3F3F3} 
Bone\_Clavicula\_L & 94.5$\pm$0.8 & 0.60$\pm$0.10 & 96.6$\pm$1.8 & 1.76$\pm$7.40 & 95.2$\pm$0.9 & 0.45$\pm$0.11 & 99.5 \\
\rowcolor[HTML]{F3F3F3} 
Bone\_Clavicula\_R & 98.4$\pm$16.1 & 1.52$\pm$0.19 & 95.5$\pm$3.2 & 1.72$\pm$9.22 & 98.3$\pm$16.0 & 1.37$\pm$0.20 & {\cellcolor[HTML]{F3F3F3}} \\
Bone\_Femur\_L & 97.4$\pm$15.4 & 3.51$\pm$0.29 & 94.6$\pm$14.3 & 9.92$\pm$40.53 & 97.5$\pm$0.7 & 3.28$\pm$0.11 & 99.7 \\
Bone\_Femur\_R & 95.8$\pm$0.5 & 6.85$\pm$0.08 & 98.4$\pm$0.4 & 0.52$\pm$1.08 & 96.3$\pm$0.2 & 6.26$\pm$0.06 & {} \\
\rowcolor[HTML]{F3F3F3} 
Bone\_Hip\_L & 96.6$\pm$1.6 & 0.32$\pm$0.13 & 97.3$\pm$1.5 & 0.44$\pm$0.89 & 97.0$\pm$1.9 & 0.29$\pm$0.14 & 99.5 \\
\rowcolor[HTML]{F3F3F3} 
Bone\_Hip\_R & 95.9$\pm$31.6 & 0.34$\pm$0.10 & 98.0$\pm$0.3 & 0.20$\pm$0.45 & 97.0$\pm$31.9 & 0.27$\pm$0.11 & {\cellcolor[HTML]{F3F3F3}} \\
SpinalCord & 92.7$\pm$16.8 & 0.27$\pm$0.24 & 94.5$\pm$3.7 & 0.20$\pm$0.13 & 92.7$\pm$16.5 & 0.26$\pm$0.24 & 99.5 \\
\rowcolor[HTML]{F3F3F3} 
Musc\_GluteusMax\_L & 98.9$\pm$5.2 & 0.84$\pm$1.41 & 93.8$\pm$7.7 & 3.56$\pm$10.31 & 98.7$\pm$5.4 & 0.76$\pm$1.50 & 99.5 \\
\rowcolor[HTML]{F3F3F3} 
Musc\_GluteusMax\_R & 98.1$\pm$2.0 & 0.93$\pm$0.34 & 95.2$\pm$4.0 & 2.29$\pm$4.92 & 97.9$\pm$2.2 & 0.71$\pm$0.34 & {\cellcolor[HTML]{F3F3F3}} \\
Musc\_GluteusMed\_L & 98.2$\pm$1.5 & 0.43$\pm$0.22 & 94.0$\pm$3.0 & 0.93$\pm$1.57 & 98.4$\pm$1.5 & 0.45$\pm$0.23 & 99.7 \\
Musc\_GluteusMed\_R & 97.6$\pm$7.3 & 0.74$\pm$0.22 & 93.7$\pm$3.8 & 0.76$\pm$0.73 & 97.3$\pm$7.5 & 0.47$\pm$0.21 & {} \\
\rowcolor[HTML]{F3F3F3} 
Musc\_GluteusMin\_L & 97.1$\pm$2.3 & 0.56$\pm$0.16 & 91.9$\pm$3.0 & 0.93$\pm$1.75 & 97.3$\pm$2.2 & 0.42$\pm$0.16 & 99.7 \\
\rowcolor[HTML]{F3F3F3} 
Musc\_GluteusMin\_R & 98.0$\pm$1.1 & 0.39$\pm$0.08 & 93.0$\pm$1.7 & 0.41$\pm$0.16 & 98.2$\pm$1.1 & 0.36$\pm$0.10 & {\cellcolor[HTML]{F3F3F3}} \\
Musc\_Autochthon\_L & 94.2$\pm$0.8 & 0.37$\pm$0.11 & 95.8$\pm$1.3 & 0.38$\pm$0.15 & 93.9$\pm$0.9 & 0.32$\pm$0.12 & 99.7 \\
Musc\_Autochthon\_R & 94.6$\pm$0.8 & 0.41$\pm$0.12 & 95.8$\pm$1.2 & 0.37$\pm$0.12 & 94.8$\pm$0.8 & 0.41$\pm$0.11 & {} \\
\rowcolor[HTML]{F3F3F3} 
Musc\_Iliopsoas\_L & 94.3$\pm$19.7 & 0.37$\pm$0.18 & 90.3$\pm$9.0 & 0.50$\pm$0.86 & 93.5$\pm$19.6 & 0.36$\pm$0.19 & 99.5 \\
\rowcolor[HTML]{F3F3F3} 
Musc\_Iliopsoas\_R & 95.0$\pm$9.1 & 0.39$\pm$0.27 & 90.0$\pm$9.5 & 0.44$\pm$0.57 & 94.9$\pm$9.1 & 0.32$\pm$0.25 & {\cellcolor[HTML]{F3F3F3}} \\
Brain & 97.9$\pm$36.4 & 0.56$\pm$1.01 & 88.3$\pm$28.0 & 7.85$\pm$24.00 & 98.2$\pm$16.3 & 0.51$\pm$1.07 & 99.5 \\
\rowcolor[HTML]{F3F3F3} 
Skull & 83.1$\pm$35.4 & 3.91$\pm$0.20 & 79.5$\pm$21.0 & 1.07$\pm$2.79 & 82.5$\pm$35.4 & 3.66$\pm$0.21 & 99.7
\\ \hline

Mean & \multicolumn{1}{c}{ 96.1 } & \multicolumn{1}{c|}{ 1.46 } & \multicolumn{1}{c}{ 94.2 } & \multicolumn{1}{c|}{ 1.78 } & \multicolumn{1}{c}{ 96.2 } & \multicolumn{1}{c|}{ 1.31 } & \multicolumn{1}{c|}{ 99.6 } \\ \hline
\end{tabular}
% }
\caption{\textbar~\textbf{Organ-wise performance comparison of \ac{nnu_e5}, MultiTalent, and \ac{cln_u5} on \ac{totalseg} `Muscle' subgroup.} Organ-wise DSC (\%) and ASD (mm) of \ac{nnu_e5}, MultiTalent and \ac{cln_u5} are evaluated on \ac{totalseg} `Muscle' subgroup. \ac{cln_u5} achieves the best mean DSC and ASD.}
\label{tab:pl_totalseg_musc_ds5}
\end{table}
\clearpage

\begin{table}[htp]
\centering
\fontsize{10pt}{12pt}\selectfont
% \resizebox{\textwidth}{!}{
\begin{tabular}{|l|ll|ll|ll|r|}
\hline
 & \multicolumn{2}{c|}{\ac{nnu_e5}} & \multicolumn{2}{c|}{MultiTalent} & \multicolumn{3}{c|}{\ac{cln_u5}} \\ \cline{2-8} 
\multirow{-2}{*}{} & DSC$\uparrow$ & ASD$\downarrow$ & DSC$\uparrow$ & ASD$\downarrow$ & DSC$\uparrow$ & ASD$\downarrow$ & $\mathcal{T}\uparrow$ \\ \hline
\rowcolor[HTML]{F3F3F3} 
Bone\_Rib1\_L & 93.6$\pm$3.3 & 0.16$\pm$0.23 & 92.4$\pm$8.9 & 0.15$\pm$0.13 & 93.3$\pm$3.3 & 0.14$\pm$0.21 & {\cellcolor[HTML]{F3F3F3}96.0} \\
\rowcolor[HTML]{F3F3F3} 
Bone\_Rib2\_L & 89.9$\pm$1.7 & 0.95$\pm$0.95 & 95.4$\pm$1.5 & 0.19$\pm$0.76 & 90.2$\pm$1.5 & 0.74$\pm$1.02 &  \\
\rowcolor[HTML]{F3F3F3} 
Bone\_Rib3\_L & 94.7$\pm$17.0 & 0.91$\pm$1.06 & 94.9$\pm$3.0 & 0.13$\pm$0.20 & 94.9$\pm$17.0 & 0.85$\pm$1.08 &  \\
\rowcolor[HTML]{F3F3F3} 
Bone\_Rib4\_L & 94.5$\pm$18.9 & 0.76$\pm$1.82 & 94.9$\pm$3.8 & 0.20$\pm$0.48 & 93.9$\pm$18.7 & 0.63$\pm$1.77 &  \\
\rowcolor[HTML]{F3F3F3} 
Bone\_Rib5\_L & 94.2$\pm$29.7 & 1.52$\pm$4.61 & 91.5$\pm$15.6 & 0.42$\pm$1.23 & 94.3$\pm$29.6 & 1.06$\pm$4.53 &  \\
\rowcolor[HTML]{F3F3F3} 
Bone\_Rib6\_L & 93.2$\pm$23.9 & 1.64$\pm$3.32 & 93.0$\pm$11.4 & 0.37$\pm$0.97 & 92.8$\pm$24.1 & 1.51$\pm$3.35 &  \\
\rowcolor[HTML]{F3F3F3} 
Bone\_Rib7\_L & 94.5$\pm$20.7 & 2.71$\pm$4.08 & 93.9$\pm$5.4 & 0.33$\pm$0.50 & 95.8$\pm$20.8 & 2.36$\pm$4.01 &  \\
\rowcolor[HTML]{F3F3F3} 
Bone\_Rib8\_L & 94.6$\pm$21.1 & 4.29$\pm$4.00 & 90.4$\pm$15.0 & 0.89$\pm$2.41 & 95.2$\pm$21.1 & 4.15$\pm$4.04 &  \\
\rowcolor[HTML]{F3F3F3} 
Bone\_Rib9\_L & 94.0$\pm$19.4 & 2.83$\pm$5.21 & 89.9$\pm$16.2 & 1.32$\pm$3.61 & 94.5$\pm$19.3 & 2.74$\pm$4.83 &  \\
\rowcolor[HTML]{F3F3F3} 
Bone\_Rib10\_L & 93.0$\pm$22.9 & 1.51$\pm$6.63 & 87.5$\pm$23.7 & 2.24$\pm$5.96 & 91.9$\pm$13.2 & 1.48$\pm$6.45 &  \\
\rowcolor[HTML]{F3F3F3} 
Bone\_Rib11\_L & 93.0$\pm$22.4 & 0.36$\pm$8.01 & 87.5$\pm$23.4 & 2.55$\pm$7.91 & 92.1$\pm$12.1 & 0.34$\pm$8.12 &  \\
\rowcolor[HTML]{F3F3F3} 
Bone\_Rib12\_L & 94.2$\pm$26.2 & 0.54$\pm$0.41 & 91.5$\pm$8.3 & 1.02$\pm$4.36 & 94.7$\pm$16.3 & 0.33$\pm$0.41 &  \\
\rowcolor[HTML]{F3F3F3} 
Bone\_Rib1\_R & 91.2$\pm$5.6 & 0.11$\pm$0.17 & 94.0$\pm$2.6 & 0.15$\pm$0.17 & 91.8$\pm$5.6 & 0.14$\pm$0.15 &  \\
\rowcolor[HTML]{F3F3F3} 
Bone\_Rib2\_R & 94.5$\pm$3.5 & 0.23$\pm$0.94 & 95.1$\pm$3.4 & 0.14$\pm$0.41 & 94.6$\pm$3.4 & 0.09$\pm$0.91 &  \\
\rowcolor[HTML]{F3F3F3} 
Bone\_Rib3\_R & 92.8$\pm$9.1 & 0.48$\pm$0.75 & 93.7$\pm$5.8 & 0.20$\pm$0.38 & 93.7$\pm$9.1 & 0.34$\pm$1.14 &  \\
\rowcolor[HTML]{F3F3F3} 
Bone\_Rib4\_R & 90.5$\pm$18.8 & 0.83$\pm$2.02 & 94.4$\pm$7.4 & 0.10$\pm$0.10 & 90.4$\pm$18.6 & 0.73$\pm$1.92 &  \\
\rowcolor[HTML]{F3F3F3} 
Bone\_Rib5\_R & 90.3$\pm$26.5 & 1.70$\pm$2.42 & 89.7$\pm$20.6 & 0.72$\pm$2.36 & 90.7$\pm$16.4 & 1.49$\pm$2.51 &  \\
\rowcolor[HTML]{F3F3F3} 
Bone\_Rib6\_R & 93.4$\pm$18.9 & 1.52$\pm$2.45 & 89.6$\pm$18.0 & 1.05$\pm$3.01 & 93.4$\pm$13.0 & 1.38$\pm$2.54 &  \\
\rowcolor[HTML]{F3F3F3} 
Bone\_Rib7\_R & 94.2$\pm$21.0 & 1.56$\pm$3.51 & 90.7$\pm$16.5 & 0.77$\pm$1.61 & 95.5$\pm$21.3 & 1.57$\pm$3.36 &  \\
\rowcolor[HTML]{F3F3F3} 
Bone\_Rib8\_R & 95.5$\pm$18.3 & 1.88$\pm$4.08 & 91.8$\pm$10.0 & 0.81$\pm$1.83 & 95.0$\pm$18.0 & 1.78$\pm$4.22 &  \\
\rowcolor[HTML]{F3F3F3} 
Bone\_Rib9\_R & 95.9$\pm$21.4 & 2.48$\pm$5.16 & 91.7$\pm$11.6 & 1.21$\pm$2.97 & 96.3$\pm$21.6 & 2.25$\pm$3.18 &  \\
\rowcolor[HTML]{F3F3F3} 
Bone\_Rib10\_R & 96.3$\pm$23.3 & 2.50$\pm$7.23 & 90.6$\pm$18.4 & 1.33$\pm$4.17 & 95.9$\pm$23.3 & 2.30$\pm$7.41 &  \\
\rowcolor[HTML]{F3F3F3} 
Bone\_Rib11\_R & 96.4$\pm$22.8 & 1.85$\pm$6.95 & 90.4$\pm$18.2 & 1.50$\pm$5.23 & 97.5$\pm$22.7 & 1.71$\pm$6.70 &  \\
\rowcolor[HTML]{F3F3F3} 
Bone\_Rib12\_R & 97.1$\pm$27.5 & 0.63$\pm$0.07 & 89.5$\pm$13.9 & 1.32$\pm$3.03 & 97.4$\pm$27.5 & 0.46$\pm$0.10 &  \\
Bone\_Sternum & 94.1$\pm$5.8 & 0.63$\pm$0.55 & 94.9$\pm$2.7 & 0.36$\pm$0.91 & 95.5$\pm$5.7 & 0.35$\pm$0.55 & {99.7} \\
\rowcolor[HTML]{F3F3F3} 
Bone\_CostalCartilages & 88.7$\pm$5.0 & 0.18$\pm$0.74 & 91.2$\pm$3.2 & 0.44$\pm$0.59 & 88.6$\pm$5.0 & 0.16$\pm$0.74 & {\cellcolor[HTML]{F3F3F3}99.5}
\\ \hline

Mean & \multicolumn{1}{c}{ 93.6 } & \multicolumn{1}{c|}{ 1.34 } & \multicolumn{1}{c}{ 91.9 } & \multicolumn{1}{c|}{ 0.77 } & \multicolumn{1}{c}{ 93.8 } & \multicolumn{1}{c|}{ 1.20 } & \multicolumn{1}{c|}{ 98.4 } \\ \hline
\end{tabular}
% }
\caption{\textbar~\textbf{Organ-wise performance comparison of \ac{nnu_e5}, MultiTalent, and \ac{cln_u5} on \ac{totalseg} `Rib' subgroup.} Organ-wise DSC (\%) and ASD (mm) of \ac{nnu_e5}, MultiTalent and \ac{cln_u5} are evaluated on \ac{totalseg} `Rib' subgroup. \ac{cln_u5} achieves the best mean DSC.}
\label{tab:pl_totalseg_ribs_ds5}
\end{table}
\clearpage

\begin{table}[htp]
\centering
\fontsize{10pt}{12pt}\selectfont
% \resizebox{\textwidth}{!}{
\begin{tabular}{|l|ll|ll|ll|r|}
\hline
 & \multicolumn{2}{c|}{\ac{nnu_e5}} & \multicolumn{2}{c|}{MultiTalent} & \multicolumn{3}{c|}{\ac{cln_u5}} \\ \cline{2-8} 
\multirow{-2}{*}{} & DSC$\uparrow$ & ASD$\downarrow$ & DSC$\uparrow$ & ASD$\downarrow$ & DSC$\uparrow$ & ASD$\downarrow$ & $\mathcal{T}\uparrow$ \\ \hline
\rowcolor[HTML]{F3F3F3} 
Bone\_Sacrum & 93.4$\pm$1.8 & 0.25$\pm$0.13 & 95.0$\pm$2.2 & 0.48$\pm$0.27 & 93.9$\pm$1.9 & 0.19$\pm$0.14 & {\cellcolor[HTML]{F3F3F3}99.0} \\
Bone\_Vert\_C1 & 94.5$\pm$20.3 & 0.25$\pm$0.53 & 94.3$\pm$4.2 & 0.42$\pm$0.53 & 95.3$\pm$10.2 & 0.23$\pm$0.50 & {96.0} \\
Bone\_Vert\_C2 & 98.0$\pm$20.7 & 0.31$\pm$3.04 & 93.2$\pm$20.1 & 0.09$\pm$0.08 & 97.9$\pm$10.5 & 0.14$\pm$0.47 &  \\
Bone\_Vert\_C3 & 98.1$\pm$23.4 & 0.16$\pm$3.22 & 94.8$\pm$10.3 & 0.28$\pm$0.64 & 98.0$\pm$15.5 & 0.16$\pm$3.18 &  \\
Bone\_Vert\_C4 & 97.0$\pm$23.4 & 0.34$\pm$3.60 & 92.1$\pm$20.0 & 0.60$\pm$1.99 & 96.6$\pm$19.6 & 0.30$\pm$3.54 &  \\
Bone\_Vert\_C5 & 96.8$\pm$17.5 & 0.22$\pm$1.62 & 88.7$\pm$22.3 & 0.26$\pm$0.62 & 97.8$\pm$17.4 & 0.21$\pm$1.63 &  \\
Bone\_Vert\_C6 & 95.0$\pm$10.6 & 0.60$\pm$0.93 & 96.9$\pm$4.6 & 0.16$\pm$0.33 & 96.0$\pm$10.5 & 0.45$\pm$0.93 &  \\
Bone\_Vert\_C7 & 95.2$\pm$17.5 & 0.41$\pm$0.86 & 96.5$\pm$5.8 & 0.19$\pm$0.45 & 95.3$\pm$13.1 & 0.18$\pm$1.00 &  \\
Bone\_Vert\_L1 & 95.7$\pm$12.1 & 1.27$\pm$0.98 & 97.1$\pm$3.1 & 0.14$\pm$0.30 & 94.9$\pm$12.1 & 1.19$\pm$0.98 &  \\
Bone\_Vert\_L2 & 94.8$\pm$18.2 & 0.29$\pm$1.09 & 97.4$\pm$1.7 & 0.11$\pm$0.21 & 93.7$\pm$12.3 & 0.18$\pm$0.95 &  \\
Bone\_Vert\_L3 & 96.0$\pm$16.1 & 0.24$\pm$1.09 & 97.0$\pm$1.8 & 0.13$\pm$0.16 & 96.9$\pm$16.2 & 0.18$\pm$1.06 &  \\
Bone\_Vert\_L4 & 94.1$\pm$14.3 & 0.43$\pm$0.41 & 95.7$\pm$6.4 & 0.22$\pm$0.39 & 94.2$\pm$14.2 & 0.23$\pm$0.41 &  \\
Bone\_Vert\_L5 & 92.9$\pm$17.3 & 0.21$\pm$1.49 & 94.6$\pm$9.5 & 0.31$\pm$0.70 & 93.9$\pm$17.4 & 0.19$\pm$1.43 &  \\
Bone\_Vert\_S1 & 96.3$\pm$23.8 & 0.20$\pm$2.10 & 92.0$\pm$14.2 & 0.42$\pm$0.96 & 97.3$\pm$18.9 & 0.19$\pm$1.22 &  \\
Bone\_Vert\_T1 & 96.3$\pm$23.5 & 0.15$\pm$1.28 & 92.5$\pm$13.0 & 0.41$\pm$0.94 & 95.9$\pm$13.5 & 0.15$\pm$1.37 &  \\
Bone\_Vert\_T2 & 98.0$\pm$5.2 & 0.48$\pm$0.74 & 88.6$\pm$22.0 & 0.59$\pm$1.38 & 97.7$\pm$5.4 & 0.32$\pm$0.76 &  \\
Bone\_Vert\_T3 & 97.0$\pm$2.7 & 0.48$\pm$0.20 & 90.4$\pm$17.1 & 0.64$\pm$1.58 & 97.9$\pm$2.6 & 0.46$\pm$0.21 &  \\
Bone\_Vert\_T4 & 89.6$\pm$17.0 & 1.12$\pm$0.21 & 91.2$\pm$16.9 & 0.51$\pm$1.50 & 90.5$\pm$8.9 & 1.05$\pm$0.20 &  \\
Bone\_Vert\_T5 & 90.7$\pm$22.9 & 0.92$\pm$0.38 & 93.6$\pm$15.8 & 0.42$\pm$1.73 & 90.4$\pm$23.1 & 0.88$\pm$0.39 &  \\
Bone\_Vert\_T6 & 86.3$\pm$28.3 & 1.15$\pm$0.07 & 92.8$\pm$15.8 & 0.48$\pm$2.13 & 85.4$\pm$28.1 & 1.04$\pm$0.06 &  \\
Bone\_Vert\_T7 & 96.8$\pm$1.0 & 1.58$\pm$0.04 & 89.9$\pm$17.5 & 0.37$\pm$1.00 & 97.1$\pm$1.0 & 1.48$\pm$0.06 &  \\
Bone\_Vert\_T8 & 91.5$\pm$13.0 & 1.08$\pm$0.40 & 84.9$\pm$24.3 & 0.18$\pm$0.22 & 91.6$\pm$13.0 & 0.93$\pm$0.16 &  \\
Bone\_Vert\_T9 & 94.6$\pm$44.2 & 0.53$\pm$0.23 & 94.4$\pm$4.6 & 0.08$\pm$0.03 & 94.3$\pm$14.4 & 0.42$\pm$0.24 &  \\
Bone\_Vert\_T10 & 97.6$\pm$29.9 & 0.36$\pm$2.18 & 95.8$\pm$0.9 & 0.10$\pm$0.07 & 97.5$\pm$13.0 & 0.38$\pm$1.32 &  \\
Bone\_Vert\_T11 & 95.1$\pm$19.4 & 0.25$\pm$1.64 & 94.7$\pm$5.5 & 0.22$\pm$0.46 & 95.1$\pm$12.4 & 0.22$\pm$1.67 &  \\
Bone\_Vert\_T12 & 97.2$\pm$16.3 & 0.32$\pm$1.30 & 84.3$\pm$27.3 & 0.24$\pm$0.34 & 97.5$\pm$16.0 & 0.26$\pm$1.35 &
\\ \hline

Mean & \multicolumn{1}{c}{ 94.9 } & \multicolumn{1}{c|}{ 0.52 } & \multicolumn{1}{c}{ 93.0 } & \multicolumn{1}{c|}{ 0.31 } & \multicolumn{1}{c}{ 95.1 } & \multicolumn{1}{c|}{ 0.45 } & \multicolumn{1}{c|}{ 97.5 } \\ \hline
\end{tabular}
% }
\caption{\textbar~\textbf{Organ-wise performance comparison of \ac{nnu_e5}, MultiTalent, and \ac{cln_u5} on \ac{totalseg} `Vertebrae' subgroup.} Organ-wise DSC (\%) and ASD (mm) of \ac{nnu_e5}, MultiTalent and \ac{cln_u5} are evaluated on \ac{totalseg} `Vertebrae' subgroup. \ac{cln_u5} achieves the best mean DSC.}
\label{tab:pl_totalseg_vert_ds5}
\end{table}
\clearpage

\begin{table}[htp]
\centering
\fontsize{10pt}{12pt}\selectfont
% \resizebox{\textwidth}{!}{
\begin{tabular}{|l|ll|ll|ll|r|}
\hline
 & \multicolumn{2}{c|}{\ac{nnu_e5}} & \multicolumn{2}{c|}{MultiTalent} & \multicolumn{3}{c|}{\ac{cln_u5}} \\ \cline{2-8} 
\multirow{-2}{*}{} & DSC$\uparrow$ & ASD$\downarrow$ & DSC$\uparrow$ & ASD$\downarrow$ & DSC$\uparrow$ & ASD$\downarrow$ & $\mathcal{T}\uparrow$ \\ \hline
\rowcolor[HTML]{F3F3F3} 
BrainStem & 93.7$\pm$1.5 & 0.32$\pm$0.10 & 87.2$\pm$2.5 & 0.84$\pm$0.26 & 92.9$\pm$1.6 & 0.23$\pm$0.11 & 99.5 \\
Eye\_L & 94.8$\pm$1.3 & 0.17$\pm$0.08 & 89.5$\pm$2.9 & 0.40$\pm$0.12 & 93.6$\pm$1.3 & 0.14$\pm$0.08 & 99.0 \\
Eye\_R & 93.2$\pm$4.2 & 0.24$\pm$0.28 & 90.0$\pm$2.5 & 1.43$\pm$2.58 & 95.3$\pm$4.3 & 0.28$\pm$0.29 & {} \\
\rowcolor[HTML]{F3F3F3} 
Lens\_L & 80.1$\pm$9.8 & 0.25$\pm$0.18 & 77.9$\pm$6.3 & 0.23$\pm$0.14 & 80.4$\pm$9.8 & 0.21$\pm$0.17 & 96.0 \\
\rowcolor[HTML]{F3F3F3} 
Lens\_R & 79.7$\pm$9.2 & 0.33$\pm$0.43 & 80.3$\pm$5.6 & 0.21$\pm$0.09 & 82.0$\pm$9.3 & 0.41$\pm$0.43 & {\cellcolor[HTML]{F3F3F3}} \\
OpticNerve\_L & 80.3$\pm$8.0 & 0.29$\pm$0.28 & 67.3$\pm$8.7 & 1.11$\pm$1.78 & 81.7$\pm$8.1 & 0.31$\pm$0.30 & 99.0 \\
OpticNerve\_R & 84.1$\pm$6.4 & 0.20$\pm$0.21 & 68.1$\pm$7.0 & 0.52$\pm$0.15 & 86.5$\pm$6.2 & 0.17$\pm$0.20 & {} \\
\rowcolor[HTML]{F3F3F3} 
Chiasm & 71.6$\pm$12.9 & 0.26$\pm$0.13 & 42.9$\pm$18.6 & 23.27$\pm$47.95 & 71.9$\pm$13.1 & 0.23$\pm$0.15 & 96.0 \\
TemporalLobe\_L & 94.7$\pm$1.2 & 0.24$\pm$0.08 & 85.6$\pm$7.0 & 1.93$\pm$0.94 & 95.3$\pm$1.3 & 0.22$\pm$0.09 & 99.5 \\
TemporalLobe\_R & 94.8$\pm$1.4 & 0.26$\pm$0.09 & 84.1$\pm$6.0 & 2.02$\pm$0.83 & 93.5$\pm$1.6 & 0.23$\pm$0.11 & {} \\
\rowcolor[HTML]{F3F3F3} 
Glnd\_Pituitary & 84.5$\pm$6.4 & 0.22$\pm$0.21 & 52.6$\pm$23.3 & 1.04$\pm$0.65 & 85.6$\pm$6.4 & 0.16$\pm$0.21 & 99.0 \\
Glnd\_Parotid\_L & 93.3$\pm$1.9 & 0.35$\pm$0.16 & 83.0$\pm$5.6 & 1.19$\pm$0.58 & 91.7$\pm$1.7 & 0.29$\pm$0.15 & 99.5 \\
Glnd\_Parotid\_R & 92.5$\pm$3.4 & 0.50$\pm$0.52 & 84.3$\pm$4.4 & 1.20$\pm$0.55 & 96.0$\pm$1.3 & 0.42$\pm$0.50 & {} \\
\rowcolor[HTML]{F3F3F3} 
Ear\_Inner\_L & 67.0$\pm$9.5 & 0.66$\pm$0.37 & 83.1$\pm$2.7 & 0.50$\pm$0.12 & 69.3$\pm$9.4 & 0.61$\pm$0.36 & 99.5 \\
\rowcolor[HTML]{F3F3F3} 
Ear\_Inner\_R & 64.3$\pm$9.3 & 0.66$\pm$0.30 & 86.8$\pm$2.7 & 0.33$\pm$0.11 & 63.8$\pm$9.4 & 0.75$\pm$0.31 & {\cellcolor[HTML]{F3F3F3}} \\
Ear\_Mid\_L & 90.4$\pm$3.7 & 0.07$\pm$0.04 & 75.2$\pm$15.7 & 1.30$\pm$1.14 & 90.6$\pm$3.6 & 0.07$\pm$0.03 & 99.5 \\
Ear\_Mid\_R & 90.2$\pm$3.3 & 0.08$\pm$0.06 & 81.2$\pm$7.0 & 1.69$\pm$2.60 & 92.1$\pm$3.4 & 0.07$\pm$0.06 & {} \\
\rowcolor[HTML]{F3F3F3} 
TMJ\_L & 84.4$\pm$9.5 & 0.31$\pm$0.23 & 78.1$\pm$6.8 & 0.79$\pm$0.34 & 82.5$\pm$9.3 & 0.24$\pm$0.22 & 98.0 \\
\rowcolor[HTML]{F3F3F3} 
TMJ\_R & 84.1$\pm$7.6 & 0.33$\pm$0.20 & 75.8$\pm$6.7 & 1.55$\pm$2.24 & 84.3$\pm$7.7 & 0.33$\pm$0.21 & {\cellcolor[HTML]{F3F3F3}} \\
SpinalCord & 91.5$\pm$2.9 & 0.36$\pm$0.19 & 81.4$\pm$3.2 & 0.61$\pm$0.14 & 90.8$\pm$3.1 & 0.33$\pm$0.21 & 99.0 \\
\rowcolor[HTML]{F3F3F3} 
Bone\_Mandible\_L & 95.7$\pm$2.1 & 0.17$\pm$0.08 & 91.4$\pm$1.9 & 0.37$\pm$0.13 & 97.5$\pm$2.0 & 0.15$\pm$0.07 & 99.7 \\
\rowcolor[HTML]{F3F3F3} 
Bone\_Mandible\_R & 95.7$\pm$2.5 & 0.17$\pm$0.08 & 91.3$\pm$1.1 & 0.36$\pm$0.10 & 95.6$\pm$2.6 & 0.13$\pm$0.09 & {\cellcolor[HTML]{F3F3F3}}

\\ \hline

Mean & \multicolumn{1}{c}{ 86.4 } & \multicolumn{1}{c|}{ 0.29 } & \multicolumn{1}{c}{ 79.0 } & \multicolumn{1}{c|}{ 1.95 } & \multicolumn{1}{c}{ 87.0 } & \multicolumn{1}{c|}{ 0.27 } & \multicolumn{1}{c|}{ 98.7 } \\ \hline
\end{tabular}
% }
\caption{\textbar~\textbf{Organ-wise performance comparison of \ac{nnu_e5}, MultiTalent, and \ac{cln_u5} on \ac{structseg}.} Organ-wise DSC (\%) and ASD (mm) of \ac{nnu_e5}, MultiTalent and \ac{cln_u5} are evaluated on \ac{structseg}. \ac{cln_u5} achieves the best mean DSC and ASD.}
\label{tab:pl_structseg_ds5}
\end{table}
\clearpage

\begin{table}[htp]
\centering
\fontsize{10pt}{12pt}\selectfont
% \resizebox{\textwidth}{!}{
\begin{tabular}{|l|ll|ll|ll|r|}
\hline
 & \multicolumn{2}{c|}{\ac{nnu_e5}} & \multicolumn{2}{c|}{MultiTalent} & \multicolumn{3}{c|}{\ac{cln_u5}} \\ \cline{2-8} 
\multirow{-2}{*}{} & DSC$\uparrow$ & ASD$\downarrow$ & DSC$\uparrow$ & ASD$\downarrow$ & DSC$\uparrow$ & ASD$\downarrow$ & $\mathcal{T}\uparrow$ \\ \hline
\rowcolor[HTML]{F3F3F3} 
Eso & 88.2$\pm$3.2 & 0.35$\pm$0.16 & 83.1$\pm$8.5 & 1.17$\pm$0.98 & 90.4$\pm$3.0 & 0.31$\pm$0.14 & 99.5 \\
Heart & 94.7$\pm$14.9 & 0.39$\pm$0.20 & 94.3$\pm$1.0 & 3.44$\pm$3.79 & 94.5$\pm$14.6 & 0.37$\pm$0.17 & 99.0 \\
\rowcolor[HTML]{F3F3F3} 
Trachea & 92.2$\pm$5.8 & 0.30$\pm$0.09 & 90.7$\pm$3.5 & 0.67$\pm$0.39 & 93.8$\pm$5.9 & 0.28$\pm$0.10 & 99.5 \\
A\_Aorta & 95.2$\pm$16.6 & 0.32$\pm$0.84 & 94.6$\pm$0.8 & 0.47$\pm$0.11 & 96.2$\pm$16.6 & 0.31$\pm$0.84 & 99.7
\\ \hline

Mean & \multicolumn{1}{c}{ 92.6 } & \multicolumn{1}{c|}{ 0.34 } & \multicolumn{1}{c}{ 90.7 } & \multicolumn{1}{c|}{ 1.44 } & \multicolumn{1}{c}{ 93.7 } & \multicolumn{1}{c|}{ 0.32 } & \multicolumn{1}{c|}{ 99.4 } \\ \hline
\end{tabular}
% }
\caption{\textbar~\textbf{Organ-wise performance comparison of \ac{nnu_e5}, MultiTalent, and \ac{cln_u5} on \ac{segthor}.} Organ-wise DSC (\%) and ASD (mm) of \ac{nnu_e5}, MultiTalent and \ac{cln_u5} are evaluated on \ac{segthor}. \ac{cln_u5} achieves the best mean DSC and ASD.}
\label{tab:pl_segthor_ds5}
\end{table}
\clearpage

\begin{table}[htp]
\centering
\fontsize{10pt}{12pt}\selectfont
% \resizebox{\textwidth}{!}{
\begin{tabular}{|l|ll|ll|ll|r|}
\hline
 & \multicolumn{2}{c|}{\ac{nnu_e5}} & \multicolumn{2}{c|}{MultiTalent} & \multicolumn{3}{c|}{\ac{cln_u5}} \\ \cline{2-8} 
\multirow{-2}{*}{} & DSC$\uparrow$ & ASD$\downarrow$ & DSC$\uparrow$ & ASD$\downarrow$ & DSC$\uparrow$ & ASD$\downarrow$ & $\mathcal{T}\uparrow$ \\ \hline
\rowcolor[HTML]{F3F3F3} 
Liver & 98.1$\pm$14.5 & 0.83$\pm$0.98 & 97.3$\pm$3.4 & 0.74$\pm$1.11 & 98.3$\pm$5.8 & 0.81$\pm$1.00 & 99.5 \\
Kidney\_R & 92.4$\pm$16.9 & 1.81$\pm$0.74 & 94.3$\pm$9.2 & 3.40$\pm$9.09 & 94.3$\pm$7.1 & 1.44$\pm$0.76 & 99.7 \\
Kidney\_L & 92.8$\pm$16.9 & 1.27$\pm$0.74 & 94.2$\pm$9.6 & 4.22$\pm$8.64 & 92.9$\pm$6.7 & 1.18$\pm$0.69 & {} \\
\rowcolor[HTML]{F3F3F3} 
Spleen & 97.9$\pm$15.6 & 0.30$\pm$0.37 & 97.1$\pm$3.4 & 0.45$\pm$0.89 & 98.0$\pm$6.6 & 0.19$\pm$0.37 & 99.5 \\
Pancreas & 91.6$\pm$17.2 & 0.80$\pm$0.69 & 89.0$\pm$4.8 & 0.98$\pm$0.68 & 92.4$\pm$7.0 & 0.72$\pm$0.38 & 99.5 \\
\rowcolor[HTML]{F3F3F3} 
A\_Aorta & 96.7$\pm$16.5 & 0.21$\pm$0.95 & 94.5$\pm$8.0 & 1.58$\pm$3.43 & 97.1$\pm$16.5 & 0.18$\pm$0.83 & 99.7 \\
V\_VenaCava\_I & 88.8$\pm$10.1 & 1.08$\pm$1.03 & 90.3$\pm$10.2 & 0.83$\pm$1.11 & 88.6$\pm$9.9 & 1.12$\pm$0.98 & 99.0 \\
\rowcolor[HTML]{F3F3F3} 
Glnd\_Adrenal\_R & 85.9$\pm$12.3 & 0.39$\pm$0.37 & 84.3$\pm$7.0 & 0.44$\pm$0.53 & 87.9$\pm$13.2 & 0.35$\pm$0.39 & 96.0 \\
\rowcolor[HTML]{F3F3F3} 
Glnd\_Adrenal\_L & 88.0$\pm$13.3 & 0.26$\pm$1.16 & 85.9$\pm$6.1 & 0.34$\pm$0.19 & 87.7$\pm$12.5 & 0.21$\pm$0.38 & {\cellcolor[HTML]{F3F3F3}} \\
GallBladder & 80.2$\pm$24.7 & 2.16$\pm$0.83 & 81.0$\pm$23.4 & 2.06$\pm$2.84 & 83.1$\pm$8.7 & 2.12$\pm$0.83 & 99.5 \\
\rowcolor[HTML]{F3F3F3} 
Eso & 84.4$\pm$3.1 & 1.70$\pm$0.15 & 84.1$\pm$15.4 & 1.93$\pm$3.34 & 86.0$\pm$3.0 & 1.61$\pm$0.14 & 99.7 \\
Stomach & 91.7$\pm$16.4 & 1.24$\pm$0.67 & 89.8$\pm$19.8 & 2.09$\pm$4.22 & 92.4$\pm$6.5 & 1.17$\pm$0.69 & 99.5 \\
\rowcolor[HTML]{F3F3F3} 
Duodenum & 79.8$\pm$25.9 & 2.71$\pm$1.29 & 79.0$\pm$16.9 & 4.77$\pm$8.97 & 81.0$\pm$16.1 & 2.39$\pm$1.18 & 99.5
\\ \hline

Mean & \multicolumn{1}{c}{ 89.9 } & \multicolumn{1}{c|}{ 1.14 } & \multicolumn{1}{c}{ 89.3 } & \multicolumn{1}{c|}{ 1.83 } & \multicolumn{1}{c}{ 90.7 } & \multicolumn{1}{c|}{ 1.04 } & \multicolumn{1}{c|}{ 99.2 } \\ \hline
\end{tabular}
% }
\caption{\textbar~\textbf{Organ-wise performance comparison of \ac{nnu_e5}, MultiTalent, and \ac{cln_u5} on \ac{flare}.} Organ-wise DSC (\%) and ASD (mm) of \ac{nnu_e5}, MultiTalent and \ac{cln_u5} are evaluated on \ac{flare}. \ac{cln_u5} achieves the best mean DSC and ASD.}
\label{tab:pl_flare_ds5}
\end{table}
\clearpage
\begin{table}[htp]
\centering
\fontsize{10pt}{12pt}\selectfont
% \resizebox{\textwidth}{!}{
\begin{tabular}{|l|ll|ll|ll|r|}
\hline
 & \multicolumn{2}{c|}{\ac{nnu_e5}} & \multicolumn{2}{c|}{MultiTalent} & \multicolumn{3}{c|}{\ac{cln_u5}} \\ \cline{2-8} 
\multirow{-2}{*}{} & DSC$\uparrow$ & ASD$\downarrow$ & DSC$\uparrow$ & ASD$\downarrow$ & DSC$\uparrow$ & ASD$\downarrow$ & $\mathcal{T}\uparrow$ \\ \hline

Kidney\_\Ac{gtv} & 86.7$\pm$9.0 & 1.18$\pm$1.06 & 79.6$\pm$20.8 & 9.94$\pm$17.66 & 87.2$\pm$9.0 & 1.03$\pm$0.98 & 96.0
\\ \hline
\end{tabular}
% }
\caption{\textbar~\textbf{Organ-wise performance comparison of \ac{nnu_e5}, MultiTalent, and \ac{cln_u5} on \ac{kits}.} Organ-wise DSC (\%) and ASD (mm) of \ac{nnu_e5}, MultiTalent and \ac{cln_u5} are evaluated on \ac{kits}. \ac{cln_u5} achieves the best mean DSC and ASD.}
\label{tab:pl_kits_ds5}
\end{table}
\clearpage
