# Supplementary material for: A Continual Learning-driven Model for Accurate and Generalizable Segmentation of Clinically Comprehensive and Fine-grained Whole-body Anatomies in CT
Source: arXiv:2503.12698 source file (2025-03-16)
Supplement: Supplementary file 10 [file external_test_results.tex]

%% external results index and analysis

%% external statistical results table
% \input{Tabs/tabs_external/tab_external_summary_clnet_nn}
